# Supplementary material for: Sorting out Lipschitz function approximation
Source: arXiv:1811.05381 source file (2019-06-11)
Supplement: Supplementary file 1 [file additional.tex]

\subsection{Additional Experiments}
